# Supplementary material for: Estimating the Probability that a Function Observed with Noise is Convex
Source: arXiv:1703.04185 source file (2018-07-27)
Supplement: Supplementary file 1 [file JianHenIJOC18Supplement.pdf]

# Online Supplement: Estimating the Probability that a Function Observed with Noise is Convex

Nanjing Jian and Shane G. Henderson
School of Operations Research and Information Engineering, Cornell University

July 25, 2018

This document is a supplement to the article "Estimating the Probability that a Function Observed with Noise is Convex" containing many of the proofs and additional material. References in this document may be internal to the document, or refer to results in the main paper. The context should make clear which is intended.

## 1 Proof of Theorem 1

First suppose that $\Gamma$ is known. Proposition 5.16 of Bernardo and Smith (2008) then establishes that

$$\Lambda_n^{-1/2}(\boldsymbol{\mu_n} - \boldsymbol{f}) \Rightarrow N(0, I), \text{ as } n \to \infty. \tag{1}$$

Using the posterior updating equations when $\Gamma$ is known, we have $\Lambda_n^{-1} = \Lambda_0^{-1} + n\Gamma^{-1}$. The square root operator is continuous over the set of positive definite matrices, so it follows that $\Lambda_n^{-1/2} = (\Lambda_0^{-1} + n\Gamma^{-1})^{1/2} \sim \sqrt{n}\,\Gamma^{-1/2}$. Slutsky's theorem applied to (1) then yields $\boldsymbol{\mu_n} - \boldsymbol{f} \to 0$ in probability as $n \to \infty$. (All norms are Euclidean in this proof.)

Now, $P(\boldsymbol{f} \in \partial\mathbb{C}) = 0$, where $\partial\mathbb{C}$ denotes the boundary of $\mathbb{C}$, since $\boldsymbol{f}$ has a density and $\partial\mathbb{C}$ is a union of a finite number of lower-dimensional faces. Thus, it is sufficient to consider the cases (i) $\boldsymbol{f} \in \mathbb{C}^\circ$, the interior of $\mathbb{C}$, which corresponds to the set of strictly convex vectors (see Section 2 of this supplement), and (ii) $\boldsymbol{f} \notin \mathbb{C}$.

On the event $\boldsymbol{f} \notin \mathbb{C}$, we can strictly separate the point $\boldsymbol{f}$ from $\mathbb{C}$ by a hyperplane. Hence we can define a random variable $D_{\boldsymbol{f}} > 0$ such that on the event $\boldsymbol{f} \notin \mathbb{C}$, all points in $\mathbb{C}$ are at least a distance $D_{\boldsymbol{f}}$ from $\boldsymbol{f}$. (Arbitrarily define $D_{\boldsymbol{f}} = 1$ on the event $\boldsymbol{f} \in \mathbb{C}$.) Let $Z \sim N(0, I)$ be a standard normal random vector, defined on the same probability space as all other random variables, and independent of all else. On the event $\boldsymbol{f} \notin \mathbb{C}$, and using the fact that $\boldsymbol{f}$ has a normal posterior distribution with parameters $\boldsymbol{\mu_n}$ and $\Lambda_n$,

$$\begin{aligned} p_n - \mathbb{1}\{\boldsymbol{f} \in \mathbb{C}\} &= P(\boldsymbol{f} \in \mathbb{C}|\mathscr{A}_n) - 0 \\ &= P(\boldsymbol{\mu_n} + \Lambda_n^{1/2} Z \in \mathbb{C}|\mathscr{A}_n) \\ &\leq P(\|\boldsymbol{\mu_n} + \Lambda_n^{1/2} Z - \boldsymbol{f}\| \geq D_{\boldsymbol{f}}|\mathscr{A}_n) \\ &\leq P(\|\boldsymbol{\mu_n} - \boldsymbol{f}\| \geq D_{\boldsymbol{f}}/2|\mathscr{A}_n) + P(\|\Lambda_n^{1/2} Z\| \geq D_{\boldsymbol{f}}/2|\mathscr{A}_n). \end{aligned} \tag{2}$$

Consider the first random variable $R_n = P(\|\boldsymbol{\mu_n} - \boldsymbol{f}\| \geq D_{\boldsymbol{f}}/2|\mathscr{A}_n)$ in (2). Then $R_n \geq 0$ and $ER_n = P(\|\boldsymbol{\mu_n} - \boldsymbol{f}\| \geq D_{\boldsymbol{f}}/2)$. We will show that this expectation converges to 0 as $n \to \infty$, and hence by Markov's inequality, it immediately follows that $R_n \to 0$ in probability as $n \to \infty$.

To this end, since $D_{\boldsymbol{f}} > 0$, for any $\epsilon > 0$ we can find $\delta > 0$ such that $P(D_{\boldsymbol{f}} \leq \delta) \leq \epsilon$. Hence,

$$\begin{aligned} P(\|\mu_n - \boldsymbol{f}\| \geq D_{\boldsymbol{f}}/2) &= P(\|\boldsymbol{\mu_n} - \boldsymbol{f}\| \geq D_{\boldsymbol{f}}/2, D_{\boldsymbol{f}} \leq \delta) + P(\|\boldsymbol{\mu_n} - \boldsymbol{f}\| \geq D_{\boldsymbol{f}}/2, D_{\boldsymbol{f}} > \delta) \\ &\leq P(D_{\boldsymbol{f}} \leq \delta) + P(\|\boldsymbol{\mu_n} - \boldsymbol{f}\| \geq \delta/2) \\ &\leq \epsilon + P(\|\boldsymbol{\mu_n} - \boldsymbol{f}\| \geq \delta/2). \end{aligned} \tag{3}$$

But $\|\boldsymbol{\mu_n} - \boldsymbol{f}\| \to 0$ as $n \to \infty$ in probability, so the second term in (3) converges to 0 as $n \to \infty$, and since $\epsilon > 0$ was arbitrary, we see that $ER_n \to 0$ as $n \to \infty$.

A similar approach works for the second term, $R'_n = P(\|\Lambda_n^{1/2}Z\| \geq D_{\boldsymbol{f}}/2|\mathscr{A}_n)$. Again, $R'_n$ is non-negative, so that if its expectation $P(\|\Lambda_n^{1/2}Z\| \geq D_{\boldsymbol{f}}/2) \to 0$ as $n \to \infty$, then $R'_n$ also converges to 0 in probability. As before, for any $\epsilon > 0$ we can find $\delta > 0$ such that $P(D_{\boldsymbol{f}} \leq \delta) \leq \epsilon$. Hence, as in (3)

$$P(\|\Lambda_n^{1/2}Z\| \geq D_{\boldsymbol{f}}/2) \leq \epsilon + P(\|\Lambda_n^{1/2}Z\| \geq \delta/2).$$

By the Cauchy-Schwarz inequality,

$$\begin{aligned} P(\|\Lambda_n^{1/2}Z\| \geq \delta/2) &\leq P(\|\Lambda_n^{1/2}\|\,\|Z\| \geq \delta/2) \\ &= P(\|Z\|^2 \geq t_n), \end{aligned}$$

where

$$t_n = \frac{\delta^2}{4}\frac{1}{\|\Lambda_n^{1/2}\|^2} \geq \frac{\delta^2}{4\|\Lambda_n\|}.$$

Now, $\Lambda_n \sim \Gamma/n$, hence $\Lambda_n^{1/2} \sim \Gamma^{1/2}/\sqrt{n}$, and so Markov's inequality gives

$$P(\|Z\|^2 \geq t_n) \leq \frac{r}{t_n} = \frac{4r\|\Lambda_n^{1/2}\|^2}{\delta^2} \to 0$$

as $n \to \infty$.

We thus conclude that (2) converges to 0 in probability as $n \to \infty$. Since $(p_n : n \geq 0)$ is a uniformly integrable martingale, it converges almost surely Williams (1991), and hence the almost sure limit is $\mathbb{1}\{\boldsymbol{f} \in C\}$.

On the other hand, on the event $\boldsymbol{f} \in \mathbb{C}^{\circ}$ we redefine $D_{\boldsymbol{f}}$ to be the radius of a ball, centered at $\boldsymbol{f}$, that is wholly contained in $\mathbb{C}$, and off this event we redefine $D_{\boldsymbol{f}} = 1$. We then find that, on the event $\boldsymbol{f} \in \mathbb{C}^{\circ}$,

$$\begin{aligned} p_n - \mathbb{1}\{\boldsymbol{f} \in \mathbb{C}\} &= P(\boldsymbol{f} \in \mathbb{C}|\mathscr{A}_n) - 1 \\ &= P(\boldsymbol{\mu_n} + \Lambda_n^{1/2}Z \in \mathbb{C}|\mathscr{A}_n) - 1 \\ &\geq P(\|\boldsymbol{\mu_n} + \Lambda_n^{1/2}Z - \boldsymbol{f}\| \leq D_{\boldsymbol{f}}|\mathscr{A}_n) - 1 \\ &\geq P(\|\boldsymbol{\mu_n} - \boldsymbol{f}\| \leq D_{\boldsymbol{f}}/2, \|\Lambda_n^{1/2}Z\| \leq D_{\boldsymbol{f}}/2|\mathscr{A}_n) - 1 \\ &\geq -P(\|\boldsymbol{\mu_n} - \boldsymbol{f}\| \geq D_{\boldsymbol{f}}/2|\mathscr{A}_n) - P(\|\Lambda_n^{1/2}Z\| \geq D_{\boldsymbol{f}}/2|\mathscr{A}_n), \end{aligned}$$

and the proof follows as in the case where $\boldsymbol{f} \notin \mathbb{C}$. This concludes the proof when $\Gamma$ is known.

Now consider the unknown variance case. From the posterior updating equations for unknown variance, $\boldsymbol{f}|\mathscr{A}_n$ follows a multivariate $t$ distribution with $\upsilon_n - r + 1$ degrees of freedom, mean $\boldsymbol{\mu_n}$, and variance $\Lambda_n = \frac{\upsilon_n - r + 1}{\upsilon_n - r - 1}\Xi_n/(\kappa_n(\upsilon_n - r + 1))$. The updating equations show that $\Xi_n$ is of order $n$, and both $\upsilon_n$ and $\kappa_n$ are of order $n$. Thus, $\Lambda_n \to \mathbf{0}$ as $n \to \infty$ a.s., where $\mathbf{0}$ is a matrix of zero components.
By Proposition 5.14 of Bernardo and Smith (2008),

$$\Lambda_n^{-1/2}(\boldsymbol{\mu_n} - \boldsymbol{f}) \Rightarrow N(0, I), \text{ as } n \to \infty. \tag{4}$$

Then this together with $\Lambda_n \to \mathbf{0}$ a.s. yields $\boldsymbol{\mu_n} - \boldsymbol{f} \to 0$ in probability as $n \to \infty$ by Slutsky's Theorem.

Again, it is sufficient to consider the cases $\boldsymbol{f} \in \mathbb{C}^{\circ}$, the interior of $\mathbb{C}$, or $\boldsymbol{f} \notin \mathbb{C}$.

As before, on the event $\boldsymbol{f} \notin \mathbb{C}$, we can define a random variable $D_{\boldsymbol{f}} > 0$ such that $D_{\boldsymbol{f}} = 1$ on the event $f \in \mathbb{C}$, and such that on the event $f \notin \mathbb{C}$, all points in $\mathbb{C}$ are at least a distance $D_{\boldsymbol{f}}$ from $\boldsymbol{f}$. Let $Z \sim N(0, I)$ be a standard normal random vector, defined on the same probability space as all other random variables, and independent of all else. On the event $\boldsymbol{f} \notin \mathbb{C}$, we use the fact that $\boldsymbol{f}|\Gamma$ has a normal posterior distribution with parameters $\boldsymbol{\mu_n}$ and $\Gamma/\kappa_n$ and take $\Gamma^{1/2}$ to be the symmetric square root of $\Gamma$. Then

$$\begin{aligned} p_n - \mathbb{1}\{\boldsymbol{f} \in \mathbb{C}\} &= P(\boldsymbol{f} \in \mathbb{C}|\mathscr{A}_n) - 0 \\ &= E(P(\boldsymbol{f} \in \mathbb{C}|\mathscr{A}_n, \Gamma)|\mathscr{A}_n) \\ &= E(P(\boldsymbol{\mu_n} + \Gamma^{1/2}Z/\sqrt{\kappa_n} \in \mathbb{C}|\mathscr{A}_n, \Gamma)|\mathscr{A}_n) \\ &\leq E(P(\|\boldsymbol{\mu_n} + \Gamma^{1/2}Z/\sqrt{\kappa_n} - \boldsymbol{f}\| \geq D_{\boldsymbol{f}}|\mathscr{A}_n, \Gamma)|\mathscr{A}_n) \\ &\leq E(P(\|\boldsymbol{\mu_n} - \boldsymbol{f}\| \geq D_{\boldsymbol{f}}/2|\mathscr{A}_n, \Gamma)|\mathscr{A}_n) \\ &\qquad + E(P(\|\Gamma^{1/2}Z/\sqrt{\kappa_n}\| \geq D_{\boldsymbol{f}}/2|\mathscr{A}_n, \Gamma)|\mathscr{A}_n) \\ &= P(\|\boldsymbol{\mu_n} - \boldsymbol{f}\| \geq D_{\boldsymbol{f}}/2|\mathscr{A}_n) + E(P(\|\Gamma^{1/2}Z/\sqrt{\kappa_n}\| \geq D_{\boldsymbol{f}}/2|\mathscr{A}_n, \Gamma)|\mathscr{A}_n). \end{aligned} \tag{5}$$

The first term in (5) converges to 0 in probability exactly as before. The second term, $R_n'$ say, is non-negative, so that if its expectation $P(\|\Gamma^{1/2}Z/\sqrt{\kappa_n}\| \geq D_{\boldsymbol{f}}/2) \to 0$ as $n \to \infty$, then $R_n'$ also converges to 0 in probability. As before, for any $\epsilon > 0$ we can find $\delta > 0$ such that $P(D_{\boldsymbol{f}} \leq \delta) \leq \epsilon$ and hence

$$E(R_n') \leq \epsilon + P(\|\Gamma^{1/2}Z/\sqrt{\kappa_n}\| \geq \delta/2). \tag{6}$$

Denoting the second term in (6) by $Q_n$, we see that

$$\begin{aligned}
Q_n &\leq P(\|Z\|\|\Gamma^{1/2}\| \geq \delta\sqrt{\kappa_n}/2) && (7)\\
&= P(\|Z\|^2 \geq \frac{\delta^2\kappa_n}{4\|\Gamma^{1/2}\|^2})\\
&\leq E(\frac{4r\|\Gamma^{1/2}\|^2}{\delta^2\kappa_n}) && (8)\\
&= \frac{4r}{\delta^2\kappa_n}E(\lambda_{\max}(\Gamma)) && (9)\\
&\leq \frac{4r}{\delta^2\kappa_n}E(\mathrm{tr}(\Gamma))\\
&= \frac{4r}{\delta^2(n+\kappa_0)}\sum_{i=1}^{r}E(\Gamma_{ii}),, && (10)
\end{aligned}$$

where $\lambda_{\max}(\Gamma)$ denotes the maximum eigenvalue of $\Gamma$, and $\mathrm{tr}(\Gamma)$ denotes the trace of $\Gamma$. The step (9) is by the definition of Euclidean norm of a real and symmetric matrix with non-negative eigenvalues. In (7) we use the sub-multiplicative property of the Euclidean norm (Golub and Van Loan 1996), and (8) is by Markov's inequality. By the Jeffery's prior of $\Gamma|\mathscr{A}_n$, conditioning on an initial sample set $\boldsymbol{y}$, $\Gamma|\mathscr{A}_0, \boldsymbol{y} \sim$ Inv-Wishart$_{\upsilon_0}(\Xi_0^{-1})$, with expectation $E(\Gamma) = (\upsilon_0 - \kappa_0 - 1)^{-1}\Xi_0^{-1}$. Thus the summation in (10) is finite, we conclude that $ER_n^{'} \to 0$ in probability, and further that $p_n - \mathbb{1}\{\boldsymbol{f} \in C\} \to 0$ in probability by (5). Again, since $(p_n : n \geq 0)$ is a uniformly integrable martingale, it converges almost surely (Williams 1991), and hence the almost-sure limit is $\mathbb{1}\{\boldsymbol{f} \in C\}$. On the other hand, in the case $\boldsymbol{f} \in \mathbb{C}^\circ$, $p_n - \mathbb{1}\{\boldsymbol{f} \in \mathbb{C}\} \geq -P(\|\boldsymbol{\mu_n} - \boldsymbol{f}\| \geq D_{\boldsymbol{f}}/2|\mathscr{A}_n) - E(P(\|\Lambda_n^{1/2}Z\| \geq D_{\boldsymbol{f}}/2|\mathscr{A}_n, \Gamma)|\mathscr{A}_n)$ and the proof follows similarly as above. □

# 2 Characterizing Strictly Convex Vectors

Here we show that the interior of $\mathbb{C}$, denoted $\mathbb{C}^\circ$, is the set of all strictly convex vectors, where $\mathbb{C}$ is defined in Definition 2 of the main paper. We repeatedly exploit the fact that $\boldsymbol{g} \in \mathbb{C}$ if and only if the linear system, (LS) in the main paper, is feasible. Throughout this section we take the points $\{\boldsymbol{x}_i : 1 \leq i \leq r\}$ as fixed. Denote the set of indices of the design points as $\mathcal{I} = \{1, 2, \ldots, r\}$. For each fixed $k \in \mathcal{I}$, consider the set $\mathcal{T}_k$ of real-valued coefficients that express $\boldsymbol{x}_k$ as a convex combination of the other points, i.e.,

$$\mathcal{T}_k = \{t \in \mathbb{R}^r : t_k = 0, t_i \in [0,1]\ i \neq k, \sum_i t_i = 1, \sum_{i=1}^{r} t_i\boldsymbol{x}_i = \boldsymbol{x}_k\}.$$

**Lemma 1.** *Given a function $g$, suppose that for each $k \in \mathcal{I}$, $\sum_{i=1}^r t_i g(\boldsymbol{x}_i) - g(\boldsymbol{x}_k) > 0$ for all $t \in \mathcal{T}_k$. Then there exists $\epsilon > 0$ such that $\sum_{i=1}^r t_i g(\boldsymbol{x}_i) - g(\boldsymbol{x}_k) \geq \epsilon > 0$ for all $k$ and all $t \in \mathcal{T}_k$.*

*Proof.* Proof. Since there are only finitely many choices for $\boldsymbol{x}_k$, we just need to show that such a bound exists for each $k \in \mathcal{I}$. So fix $k \in \mathcal{I}$. If $\mathcal{T}_k$ is a finite set, then the required bound exists by taking the minimum over a finite number of positive terms. So suppose $\mathcal{T}_k$ contains an infinite number of terms, as arises for example when multiple $\boldsymbol{x}_i$ are linearly dependent. If a positive $\epsilon$ as stated does not exist, then there is a sequence $\{t^{(n)}, n \geq 1\}$ contained in $\mathcal{T}_k$ such that $D(n) := \sum_{i=1}^r t_i^{(n)} g(\boldsymbol{x}_i) - g(\boldsymbol{x}_k) \to 0$ as $n \to \infty$. The set $\mathcal{T}_k$ is compact, so by passing to a subsequence we can assume that $t^{(n)} \to t^* \in \mathcal{T}_k$ as $n \to \infty$. Also since $D(n) \to 0$, it follows by continuity that $D^* = \sum_{i=1}^r t_i^* g(\boldsymbol{x}_i) - g(\boldsymbol{x}_k) = \lim_{n\to\infty} D(n) = 0$, which contradicts the assumption of the lemma. □ □

**Proposition 1.** *An $r$-dimensional vector $\boldsymbol{g} \in \mathbb{C}^\circ$ if and only if there exists a strictly convex function $g$ whose values on $\boldsymbol{x}$ coincide with those of $\boldsymbol{g}$, i.e. $g(\boldsymbol{x}) = \boldsymbol{g}$ for $\boldsymbol{x} = (\boldsymbol{x}_1, \boldsymbol{x}_2, \ldots, \boldsymbol{x}_r)$.*

*Proof.* Proof. First, suppose there exists a strictly convex function $g$ with $g(\boldsymbol{x}) = \boldsymbol{g}$. We want to show $\boldsymbol{g} \in \mathbb{C}^\circ$. Since $g$ is strictly convex, the strict inequalities in the statement of Lemma 1 hold for all $k \in \mathfrak{I}$ and all $t \in \mathfrak{T}_k$. Lemma 1 then implies that there exists $\epsilon > 0$ such that

$$\sum_{i=1}^{r} t_i g(\boldsymbol{x}_i) \geq g(\boldsymbol{x}_k) + \epsilon \tag{11}$$

for all $k$ and all $t \in \mathfrak{T}_k$. Consider the ball in $\mathbb{R}^r$ defined by $(\boldsymbol{y} \in \mathbb{R}^r : |\boldsymbol{y}_i| \leq \epsilon/2 \ \forall i)$, and the perturbed vector $\tilde{g} = \boldsymbol{g} + \boldsymbol{y}$ with $i$th component $g(\boldsymbol{x}_i) + \boldsymbol{y}_i$. Then for any $k \in \mathfrak{I}$ and any $t \in \mathfrak{T}_k$,

$$\begin{aligned}
\left(\sum_{i=1}^{r} t_i \tilde{g}(\boldsymbol{x}_i)\right) - \tilde{g}(\boldsymbol{x}_k) &= \left(\sum_{i=1}^{r} t_i (g(\boldsymbol{x}_i) + \boldsymbol{y}_i)\right) - (g(\boldsymbol{x}_k) + \boldsymbol{y}_k) \\
&= \sum_{i=1}^{r} t_i g(\boldsymbol{x}_i) - g(\boldsymbol{x}_k) + \left(\sum_{i=1}^{r} t_i \boldsymbol{y}_i\right) - \boldsymbol{y}_k \\
&\geq \epsilon - \max_{i=1}^{r} |\boldsymbol{y}_i| - |\boldsymbol{y}_k| \\
&\geq \epsilon - \epsilon/2 - \epsilon/2 = 0.
\end{aligned}$$

Thus all perturbed function values in the ball centered at $\boldsymbol{g}$ are convex, and it follows that $\boldsymbol{g} \in \mathbb{C}^\circ$.

Now suppose that $\boldsymbol{g} \in \mathbb{C}^\circ$. We want to show that there exists a strictly convex function, $g^*$ say, that coincides with $\boldsymbol{g}$ on $\boldsymbol{x}$. Since $\boldsymbol{g} \in \mathbb{C}$ there exists a convex function $g$ that coincides with $\boldsymbol{g}$ on $\boldsymbol{x}$. Let $h$ be an arbitrary finite-valued strictly convex function, e.g., $h(x) = \|x\|_2^2$, and let $\boldsymbol{h}$ be the restriction of $h$ to $\boldsymbol{x}$. For $\delta > 0$ sufficiently small, $\boldsymbol{g} - \delta\boldsymbol{h} \in \mathbb{C}$, since $g \in \mathbb{C}^\circ$ and $\delta\boldsymbol{h}$ is a finite vector with arbitrarily small norm for $\delta$ sufficiently small. Thus, there exists a convex function $f$ that coincides with $\boldsymbol{g} - \delta\boldsymbol{h}$ on $\boldsymbol{x}$. But then $g^* = f + \delta h$ coincides with $\boldsymbol{g}$ on $\boldsymbol{x}$, and is the sum of a convex and strictly convex function so is strictly convex. □ □

# 3 Proof of Theorem 2

First, similar to the known variance case, the distribution of $\boldsymbol{f}|\mathscr{A}_n$, being multivariate $t$, is absolutely continuous with respect to the distribution of $\boldsymbol{f}|\mathscr{A}_{n+\ell}$. Thus $E(\hat{p}_{n+\ell}|\mathscr{A}_{n+\ell}) = p_{n+\ell}$, and $\hat{p}_{n+\ell}$ is unbiased. It remains to show that $E(\hat{p}^2_{n+\ell}|\mathscr{A}_{n+\ell}) < \infty$, so that conditional on $\mathscr{A}_{n+\ell}$ the estimator has finite second moment and hence variance.

When $\Gamma$ is unknown, $\boldsymbol{f}|\mathscr{A}_n$ is distributed as multivariate $t$ centered at $\boldsymbol{\mu_n}$ with scale matrix $\Xi_n/[\kappa_n(\nu_n - r + 1)]$ and $\nu_n - r + 1$ degrees of freedom. Since $E(\hat{p}^2_{n+\ell}|\mathscr{A}_{n+\ell}) = E(\mathbb{1}\{\boldsymbol{Y} \in \mathbb{C}\}L^2_{n+\ell,n}(\boldsymbol{Y})|\mathscr{A}_{n+\ell})$, it suffices to show that $L^2_{n+\ell,n}(\boldsymbol{y})$ is bounded in $\boldsymbol{y}$ for any $n$. We will do this by showing that the ratio of an upper bound on the numerator to a lower bound of the denominator is bounded. Moreover, it suffices to obtain such a bound outside a compact set, since $t$ densities are bounded above, and are bounded below on any compact set. Hence, we need only show a bound outside a compact set $C$ that will be successively defined as we proceed.

Let $\lambda_{\max}$ be the largest eigenvalue of $\Lambda_{n+\ell} = \Xi_{n+\ell}/\kappa_{n+\ell}$. Then the squared density of $\boldsymbol{f}|\mathscr{A}_{n+\ell}$ evaluated at $\boldsymbol{y}$ is proportional to

$$\begin{aligned}
&\{1 + (\boldsymbol{y} - \boldsymbol{\mu_{n+\ell}})\Lambda^{-1}_{n+\ell}(\boldsymbol{y} - \boldsymbol{\mu_{n+\ell}})/(\nu_{n+\ell} - r + 1)\}^{-(\nu_{n+\ell}+1)} \qquad (12)\\
&\leq \{1 + (\lambda_{\max})^{-1}||\boldsymbol{y} - \boldsymbol{\mu_{n+\ell}}||^2/(\nu_{n+\ell} - r + 1)\}^{-(\nu_{n+\ell}+1)} \\
&\leq \left\{\frac{||\boldsymbol{y} - \boldsymbol{\mu_{n+\ell}}||^2}{\lambda_{\max}(\nu_{n+\ell} - r + 1)}\right\}^{-(\nu_{n+\ell}+1)} \\
&= c_1||\boldsymbol{y} - \boldsymbol{\mu_{n+\ell}}||^{-2(\nu_{n+\ell}+1)}, \qquad (13)
\end{aligned}$$

where the constant $c_1 = \{\lambda^+_{\max}(\nu_{n+\ell} - r + 1)\}^{(\nu_{n+\ell}+1)}$. This constant depends on $n$ but does not depend on $\boldsymbol{y}$. Likewise, let $\lambda_{\min}$ be the smallest eigenvalue of $\Lambda_n = \Xi_n/\kappa_n$. Then the squared density of $\boldsymbol{f}|\mathscr{A}_n$ evaluated at $\boldsymbol{y}$

is proportional to

$$\begin{aligned}
&\{1+(\boldsymbol{y}-\boldsymbol{\mu_n})\Lambda_n^{-1}(\boldsymbol{y}-\boldsymbol{\mu_n})/(\nu_n-r+1)\}^{-(\nu_n+1)}\\
&\geq \{1+\lambda_{\min}^{-1}||\boldsymbol{y}-\boldsymbol{\mu_n}||^2/(\nu_n-r+1)\}^{-(\nu_n+1)}\\
&\geq \left\{\frac{2||\boldsymbol{y}-\boldsymbol{\mu_n}||^2}{\lambda_{\min}(\nu_n-r+1)}\right\}^{-(\nu_n+1)} \qquad (14)\\
&= ||\boldsymbol{y}-\mu_n||^{-2(\nu_n+1)}, \qquad (15)
\end{aligned}$$

where the constant $c_2 = \{\lambda_{\min}(\nu_n-r+1)/2\}^{(\nu_n+1)}$. The bound (14) applies for $y$ outside the compact set $C = \{\boldsymbol{y} : \|\boldsymbol{y}-\boldsymbol{\mu_n}\|^2 \leq \lambda_{\min}(\nu_n-r+1)\}$.

Taking the ratio of (13) and (15), we have that for $\boldsymbol{y} \notin \mathbb{C}$,

$$\begin{aligned}
L^2_{n+\ell,n}(\boldsymbol{y}) &\leq \frac{c_1||\boldsymbol{y}-\boldsymbol{\mu_{n+\ell}}||^{-2(\nu_{n+\ell}+1)}}{c_2||\boldsymbol{y}-\boldsymbol{\mu_n}||^{-2(\nu_n+1)}}\\
&= \frac{c_1}{c_2}\cdot\frac{||\boldsymbol{y}-\boldsymbol{\mu_n}||^{2(\nu_n+1)}}{||\boldsymbol{y}-\boldsymbol{\mu_{n+\ell}}||^{2(\nu_{n+\ell}+1)}}\\
&= \frac{c_1}{c_2}\cdot\frac{||\boldsymbol{y}-\boldsymbol{\mu_{n+\ell}}+\boldsymbol{\mu_{n+\ell}}-\boldsymbol{\mu_n}||^{2(\nu_n+1)}}{||\boldsymbol{y}-\boldsymbol{\mu_{n+\ell}}||^{2(\nu_{n+\ell}+1)}}\\
&\leq \frac{c_1}{c_2}\cdot\frac{(||\boldsymbol{y}-\boldsymbol{\mu_{n+\ell}}||+||\boldsymbol{\mu_{n+\ell}}-\boldsymbol{\mu_n}||)^{2(\nu_n+1)}}{||\boldsymbol{y}-\boldsymbol{\mu_{n+\ell}}||^{2(\nu_{n+\ell}+1)}}\\
&\leq \frac{c_1}{c_2}\cdot 2^{2\nu_n+1}\frac{||\boldsymbol{y}-\boldsymbol{\mu_{n+\ell}}||^{2(\nu_n+1)}+||\boldsymbol{\mu_{n+\ell}}-\boldsymbol{\mu_n}||^{2(\nu_n+1)}}{||\boldsymbol{y}-\boldsymbol{\mu_{n+\ell}}||^{2(\nu_{n+\ell}+1)}}\\
&\leq \frac{c_1}{c_2}\cdot 2^{2\nu_n+1}\left\{||\boldsymbol{y}-\boldsymbol{\mu_{n+\ell}}||^{2(\nu_n-\nu_{n+\ell})}+\frac{||\boldsymbol{\mu_{n+\ell}}-\boldsymbol{\mu_n}||^{2(\nu_n+1)}}{||\boldsymbol{y}-\boldsymbol{\mu_{n+\ell}}||^{2(\nu_{n+\ell}+1)}}\right\}. \qquad (16)
\end{aligned}$$

The second to last step uses Jensen's inequality $f((a+b)/2) \leq (f(a)+f(b))/2$ on the convex function $f(x) = x^{2(\nu_n+1)}$ where $x > 0$ and $\nu_n > 0$.

Finally, for the bracketed term in (16), we enlarge the "exclusion compact set" $C$ if necessary so that $||\boldsymbol{y} - \boldsymbol{\mu_{n+\ell}}||^2 \geq 1$ for $y \notin C$ and then the first term is at most 1 since $\nu_n < \nu_{n+\ell}$, and the second term is at most $||\boldsymbol{\mu_{n+\ell}} - \boldsymbol{\mu_n}||^{2(\nu_n+1)}$. Thus the term is bounded above for any fixed $n$. □

# 4 Proof of Proposition 1

When $r = 1$, the density of $f|\mathscr{A}_n$ is $\phi_n \sim N(\boldsymbol{\mu_n}, \sigma_n^2)$. Denote the true sampling variance as $\gamma^2$, and the precision $\gamma^{-2} = \lambda$. According to the posterior updating equations in the case of known variance, we have

$$\begin{aligned}
\sigma_{n+1}^{-2} &= \sigma_n^{-2} + \lambda = \sigma_0^{-2} + (n+1)\lambda,\\
\sigma_n^{-2} &= \sigma_0^{-2} + n\lambda,\\
\boldsymbol{\mu_{n+1}} &= \sigma_{n+1}^2(\sigma_n^{-2}\boldsymbol{\mu_n} + \lambda\bar{z}),
\end{aligned}$$

where $\bar{z} \sim N(\mu, \gamma^2)$ for some constant $\mu$. Then for any $y \in \mathbb{R}$, $\ln L_{n+1,n}(y)$ is

$$\begin{aligned}
&\ln\left(\frac{\phi_{n+1}(y)}{\phi_n(y)}\right) \\
&= \ln\left(\frac{\sigma_n}{\sigma_{n+1}}\right) - \frac{(y-\boldsymbol{\mu_{n+1}})^2}{2\sigma_{n+1}^2} + \frac{(y-\boldsymbol{\mu_{n+}})^2}{2\sigma_n^2} \\
&= \frac{1}{2}\ln\left(\frac{\sigma_0^{-2}+(n+1)\lambda}{\sigma_0^{-2}+n\lambda}\right) - \frac{1}{2}(y-\boldsymbol{\mu_{n+1}})^2(\sigma_0^{-2}+(n+1)\lambda) + \frac{1}{2}(y-\boldsymbol{\mu_{n+}})^2(\sigma_0^{-2}+n\lambda) \\
&= q_n + \frac{1}{2}\left[(y-\boldsymbol{\mu_{n+}})^2(\sigma_0^{-2}+n\lambda) - (y-\boldsymbol{\mu_n}+\boldsymbol{\mu_n}-\boldsymbol{\mu_{n+1}})^2(\sigma_0^{-2}+(n+1)\lambda)\right] \\
&= q_n + \frac{1}{2}\left[-\lambda(y-\boldsymbol{\mu_{n+}})^2 - 2(\boldsymbol{\mu_n}-\boldsymbol{\mu_{n+1}})(\sigma_0^{-2}+(n+1)\lambda)(y-\boldsymbol{\mu_n}) + (\boldsymbol{\mu_n}-\boldsymbol{\mu_{n+1}})^2(\sigma_0^{-2}+(n+1)\lambda)\right] \\
&= q_n - \frac{\lambda}{2}\left\{y-\boldsymbol{\mu_n}+\frac{1}{\lambda}\left[(\boldsymbol{\mu_n}-\boldsymbol{\mu_{n+1}})(\sigma_0^{-2}+(n+1)\lambda)\right]\right\}^2 \\
&\quad - \frac{1}{2}(\boldsymbol{\mu_n}-\boldsymbol{\mu_{n+1}})^2\left[(\sigma_0^{-2}+(n+1)\lambda) - \frac{1}{\lambda}(\sigma_0^{-2}+(n+1)\lambda)^2\right],
\end{aligned}$$

where $q_n = \frac{1}{2}\ln\left(\frac{\sigma_0^{-2}+(n+1)\lambda}{\sigma_0^{-2}+n\lambda}\right)$ is a constant. Maximizing over $y$ gives

$$\begin{aligned}
\ln C_n &= \sup_y \ln\left(\frac{\phi_{n+1}(y)}{\phi_n(y)}\right) \\
&= q_n - \frac{1}{2}(\boldsymbol{\mu_n}-\boldsymbol{\mu_{n+1}})^2\left[(\sigma_0^{-2}+(n+1)\lambda) - \frac{1}{\lambda}(\sigma_0^{-2}+(n+1)\lambda)^2\right] \\
&= q_n - \frac{1}{2}(\boldsymbol{\mu_n}-\boldsymbol{\mu_{n+1}})^2\left[\sigma_{n+1}^{-2} - \frac{1}{\lambda}(\sigma_{n+1}^{-2})^2\right].
\end{aligned}$$

Here,

$$\begin{aligned}
\boldsymbol{\mu_n}-\boldsymbol{\mu_{n+1}} &= \boldsymbol{\mu_n} - \sigma_{n+1}^2(\sigma_n^{-2}\boldsymbol{\mu_n}+\lambda\bar{z}) \\
&= (1-\frac{\sigma_{n+1}^2}{\sigma_n^2})\boldsymbol{\mu_n} - \sigma_{n+1}^2\lambda\bar{z} \\
&= \boldsymbol{\mu_n}\left(1-\frac{\sigma_0^{-2}+n\lambda}{\sigma_0^{-2}+(n+1)\lambda}\right) - \sigma_{n+1}^2\lambda\bar{z} \\
&= \boldsymbol{\mu_n}\frac{\lambda}{\sigma_0^{-2}+(n+1)\lambda} - \sigma_{n+1}^2\lambda\bar{z} \\
&= \boldsymbol{\mu_n}\frac{\lambda}{\sigma_{n+1}^{-2}} - \sigma_{n+1}^2\lambda\bar{z} \\
&= \lambda\sigma_{n+1}^2(\boldsymbol{\mu_n}-\bar{z}),
\end{aligned}$$

where $\bar{z}$ is the average over the samples used to update the posterior. We have been using just one sample for the update, so $\bar{z} \sim N(\mu, \sigma^2)$, where $\sigma^2$ is the sampling variance.
Substituting, we obtain

$$\begin{aligned}
\ln C_n &= q_n - \frac{1}{2}(\boldsymbol{\mu_n}-\boldsymbol{\mu_{n+1}})^2\left[\sigma_{n+1}^{-2} - \frac{1}{\lambda}(\sigma_{n+1}^{-2})^2\right] \\
&= q_n - \frac{1}{2}\lambda^2\sigma_{n+1}^4(\boldsymbol{\mu_n}-\bar{z})^2\left[\sigma_{n+1}^{-2} - \frac{1}{\lambda}(\sigma_{n+1}^{-2})^2\right] \\
&= q_n - \frac{1}{2}\lambda^2(\boldsymbol{\mu_n}-\bar{z})^2\left[\sigma_{n+1}^2 - \frac{1}{\lambda}\right] \\
&= q_n - \frac{1}{2}\lambda^2(\boldsymbol{\mu_n}-\bar{z})^2\left[\frac{1}{\sigma_n^{-2}+\lambda} - \frac{1}{\lambda}\right].
\end{aligned}$$

Here $\boldsymbol{\mu_n} - \bar{z} = \boldsymbol{\mu_n} - (\mu - \sigma N) = \sigma N + \boldsymbol{\mu_n} - \mu$, where $N$ is a standard normal random variable, so $(\boldsymbol{\mu_n} - \bar{z})^2 = \sigma^2(N + (\boldsymbol{\mu_n} - \mu)/\sigma)^2$. Thus conditional on $\mathscr{A}_n$,

$$\begin{aligned} \ln C_n &= q_n - \frac{1}{2}\lambda^2\sigma^2(N + (\boldsymbol{\mu_n} - \mu)/\sigma)^2 \left[\frac{1}{\sigma_n^{-2} + \lambda} - \frac{1}{\lambda}\right] \\ &\sim \frac{1}{2}\left(N + \frac{\boldsymbol{\mu_n} - \mu}{\sigma}\right)^2, \end{aligned}$$

since $\lambda = \sigma^{-2}$ and $q_n \sim 0$ as $n \to \infty$. Here $N$ is a standard normal random variable, so $\ln C_n$ is distributed as a non-central chi-square with 1 degree of freedom and non-central parameter $(\boldsymbol{\mu_n} - \mu)^2/\sigma^2$; see, e.g., Glasserman (2004, p. 123). $\square$

# 5 Proof of Theorem 3

Let the density function of $X = (X_1, X_2, \ldots, X_r)$ be $\phi(\cdot)$, which is the density function of the $N(0, I)$ distribution in the known variance case, and the density of the $t_{\nu_n}(0, I)$ distribution in the unknown variance case.
Consider the transformation of $X$ into $r$ random variables $(T, Z_1, Z_2, \ldots, Z_{r-1})$ with $(X_1, X_2, \ldots, X_r) = (TZ_1, TZ_2, \ldots, TZ_r)$, where $Z = (Z_1, Z_2, \ldots, Z_r)$ lies on $S_+^{r-1}$, the upper hemisphere of the $(r-1)$ unit spherical shell $S_+^{r-1}$. Hence $Z_r = (1 - \sum_{i=1}^{r-1} Z_i^2)^{1/2}$ is non-negative and $T$ takes both positive and negative values. Let $\tilde{Z} = (Z_1, Z_2, \cdots, Z_{r-1})$. Let $A \subseteq \mathbb{R}^r$ be an arbitrary (measurable) set. Then the posterior probability that $\boldsymbol{f} \in A$ can be written as

$$\begin{aligned} P(\boldsymbol{f} \in A|\mathscr{A}_n) &= \int_{\mathbb{R}^r} \mathbb{1}\left\{\Lambda_n^{1/2}x + \mu_n \in A\right\}\phi(x)dx \\ &= \int_{S_+^{r-1}} \int_{-\infty}^{\infty} \mathbb{1}\left\{\Lambda_n^{1/2}tz + \mu_n \in A\right\}\phi(tz)\left|\det(J)\right| dt d\tilde{z}, \end{aligned} \tag{17}$$

where $J$ is the Jacobian of the transformation $(x_1, x_2, \ldots, x_r) = (tz_1, tz_2, \ldots, tz_r)$ and $\det(\cdot)$ is the determinant operator.
For $i = 1, 2, \ldots, r-1$,

$$\frac{\partial z_r}{\partial z_i} = \frac{1}{2}\left(1 - \sum_{i=1}^{r-1} z_i^2\right)^{-1/2}(-2z_i) = -\frac{z_i}{z_r},$$

so that the Jacobian matrix is

$$J = \begin{pmatrix} z_1 & t & 0 & \cdots & 0 \\ z_2 & 0 & t & \cdots & 0 \\ \vdots & \vdots & \vdots & \ddots & \vdots \\ z_{r-1} & 0 & \cdots & \cdots & t \\ z_r & -\frac{z_1 t}{z_r} & -\frac{z_2 t}{z_r} & \cdots & -\frac{z_{r-1} t}{z_r} \end{pmatrix}.$$

Its determinant can be found by expanding along the last row (leaving zero components empty) to give

$$
\begin{aligned}
\det(J) =& z_r t^{r-1}(-1)^{r+1} + \left(-\frac{z_1 t}{z_r}\right)\begin{vmatrix} z_1 & 0 & \cdots & \cdots & 0 \\ z_2 & t & & & \\ z_3 & 0 & t & & \\ \vdots & 0 & 0 & \ddots & \\ z_{r-1} & \cdots & \cdots & \cdots & t \end{vmatrix}(-1)^{r+2} + \left(-\frac{z_2 t}{z_r}\right)\begin{vmatrix} z_1 & t & & & \\ z_2 & 0 & & & \\ z_3 & 0 & t & & \\ \vdots & 0 & 0 & \ddots & \\ z_{r-1} & \cdots & \cdots & \cdots & t \end{vmatrix}(-1)^{r+3} + \\
& \left(-\frac{z_3 t}{z_r}\right)\begin{vmatrix} z_1 & t & & & \\ z_2 & 0 & t & & \\ z_3 & 0 & 0 & \cdots & \\ \vdots & 0 & 0 & \ddots & \\ z_{r-1} & \cdots & \cdots & \cdots & t \end{vmatrix}(-1)^{r+4} + \cdots + \left(-\frac{z_{r-1} t}{z_r}\right)\begin{vmatrix} z_1 & t & & & \\ z_2 & 0 & t & & \\ z_3 & 0 & 0 & t & \\ \vdots & 0 & 0 & \ddots & \\ z_{r-1} & 0 & 0 & \cdots & 0 \end{vmatrix}(-1)^{2r} \\
=& (-1)^{r+1}\left(z_r t^{r-1} + \frac{z_1 t}{z_r} z_1 t^{r-2} + \frac{z_2 t}{z_r} z_2 t^{r-2} + \cdots + \frac{z_{r-1} t}{z_r} z_{r-1} t^{r-2}\right) \\
=& (-1)^{r+1}\left(\frac{1}{z_r} t^{r-1}(z_r^2 + z_1^2 + \cdots + z_{r-1}^2)\right) \\
=& (-1)^{r+1}\frac{t^{r-1}}{z_r}.
\end{aligned}
$$

Thus, from (17),

$$P(\boldsymbol{f} \in A|\mathscr{A}_n) = \int_{S_+^{r-1}} \int_{-\infty}^{\infty} \mathbb{1}\left\{\Lambda_n^{1/2} z t + \mu_n \in A\right\} \phi(tz)\frac{|t|^{r-1}}{z_r} dt d\tilde{z}.$$

Since the set $A$ was arbitrary, we conclude that the density of $TZ$ is proportional to $\phi(tz)|t|^{r-1}/z_r$.

In the known variance case, $\phi(u) \propto e^{-\|u\|^2/2}$ ($\propto$ denotes "proportional to"), and since $\|z\| = 1$, $\phi(tz) \propto e^{-t^2/2}$. Hence the density of $TZ$ is proportional to $e^{-t^2/2}|t|^{r-1}/z_r$. This expression is separable in the two components $t$ and $\tilde{z}$, so we conclude that $T$ and $Z$ are independent, and moreover that the density of $T$ is proportional to $e^{-t^2/2}|t|^{r-1}$. The density of $T$ is an even function so $T$ is symmetric around 0, and for $v \geq 0$,

$$P(0 \leq T \leq v) \propto \int_0^v e^{-t^2/2} t^{r-1}\, dt = \int_0^{v^2} e^{-w/2} w^{r/2-1}\, dw.$$

The integrand (in $w$) is proportional to the density of a chi-squared random variable with $r$ degrees of freedom, which yields the result for the known variance case.

In the unknown variance case, $\phi(u) \propto (1 + u^T u/\nu_n)^{-(\nu_n+r)/2}$, so again $\phi(tz)$ does not depend on $z$. The rest of the argument is the same as that for known variance, where we exploit the fact that the density of an F-distributed random variable with degrees of freedom $r, \nu_n$ is proportional to

$$\frac{(rt)^{r/2}}{t(rt + \nu_n)^{r+\nu_n}}.$$

It remains to confirm that $Z$ is uniform on $S_+^{r-1}$, but this follows without calculation from the spherical symmetry of $\phi$ in both the known and unknown variance cases. □

# 6 Alternatives to the Posterior Updates

When the covariance matrix $\Gamma$ is known,the normal-normal conjugate prior (posterior) updates given in the main paper involve inverting the posterior covariance matrix $\Lambda_n$ in every iteration. An alternative method is to use the Sherman-Morrison-Woodbury formula

$$
\begin{aligned}
\boldsymbol{\mu_n} &= \mu_{n-1} + \Lambda_{n-1} s\Gamma^{-1}(I + \Lambda_{n-1} s\Gamma^{-1})^{-1}(\bar{y} - \mu_{n-1}) \\
\Lambda_n &= \Lambda_{n-1} - \Lambda_{n-1} s\Gamma^{-1}(I + \Lambda_{n-1} s\Gamma^{-1})^{-1}\Lambda_{n-1}
\end{aligned}
\tag{18}
$$

In this version, only the inverse of $(I + \Lambda_{n-1} s\Gamma^{-1})$ needs to be updated in each iteration, and the inverse of $\Lambda_{n-1}$ is not required. However, since $\Gamma$ is full rank, this update is a full rank update on $\Lambda_n$, which means the calculation still requires $O(r^3)$ math operations.

Another way to avoid repeated matrix inversions is to update the precision matrix $\Lambda_n^{-1}$ from iteration $n$ to $n+1$ instead of the covariance matrix, and to use the Cholesky factorization when performing the updates. In each iteration, the update formula is

$$\begin{aligned}
\Lambda_n^{-1} &= \Lambda_{n-1}^{-1} + s\Gamma^{-1} \\
L_n &= \mathrm{Chol}(\Lambda_n^{-1}) \\
\boldsymbol{\mu_n} &= \Lambda_n(\Lambda_{n-1}^{-1}\mu_{n-1} + s\Gamma^{-1}\bar{\boldsymbol{y}}) \\
&= L_n^T \backslash [L_n \backslash (\Lambda_{n-1}^{-1}\mu_{n-1} + s\Gamma^{-1}\bar{\boldsymbol{y}})].
\end{aligned} \tag{19}$$

Here $\mathrm{Chol}(\Lambda_n^{-1})$ is the lower-triangular Cholesky factor of $\Lambda_n^{-1}$, which is unique when $\Gamma_n^{-1}$ positive definite, and $x = A\backslash b$ means to solve the linear system $Ax = b$. In Algorithm 2, when samples with distribution $N(\boldsymbol{\mu_n}, \Lambda_n)$ are required, we can generate them by computing $\boldsymbol{\mu_n} + L_n^T\backslash\boldsymbol{Z}$, where $\boldsymbol{Z} \sim N(\mathbf{0}, I)$. This is based on the fact that $\mathrm{Chol}(\Lambda_n) = L_n^{-T}$. We are not able to find a way to directly update the Cholesky factor, so the Cholesky decomposition step is required in each iteration, which means that this method also has $O(r^3)$ complexity at each iteration.

Although these proposals do not reduce the computational complexity of the update, they allow us to do fewer matrix inversions, which makes them numerically more robust.

# References


Bernardo, José M., Adrian F. M. Smith. 2008. *Bayesian Theory*. John Wiley & Sons, Inc., 240–376. doi:10.1002/9780470316870.ch5. URL http://dx.doi.org/10.1002/9780470316870.ch5.

Glasserman, Paul. 2004. *Monte Carlo methods in financial engineering*. Springer, New York. URL http://www.amazon.com/Financial-Engineering-Stochastic-Modelling-Probability/dp/0387004513/ref=pd_sim_b_68?ie=UTF8&refRID=1AN8JXSDGMEV2RPHFC2A.

Golub, Gene H., Charles F. Van Loan. 1996. *Matrix Computations*. 3rd ed. Johns Hopkins Studies in Mathematical Sciences, The Johns Hopkins University Press. URL http://www.worldcat.org/isbn/0801854148.

Williams, D. 1991. *Probability with Martingales*. Cambridge mathematical textbooks, Cambridge University Press. URL http://books.google.com/books?id=RnOJeRpk0SEC.
